# Supplementary material for: Near Optimal Stochastic Algorithms for Finite-Sum Unbalanced Convex-Concave Minimax Optimization
Source: arXiv:2106.01761 source file (2022-01-30)
Supplement: Supplementary file 1 [file cc2.tex]

\section{CC}

 \paragraph{Case 1:} If $\eps\leq L/\sqrt{n}$, 
 L-SVRE with $K$ iterations holds that
 \begin{align*}
     {\rm Gap} \leq \frac{L}{\sqrt{p}K}. 
 \end{align*}
 We hope ${\rm Gap} \leq \eps$ which requires 
 \begin{align*}
  K\geq \dfrac{L}{\sqrt{p}\eps}.
 \end{align*}
 Then the total SFO complexity is at least
 \begin{align*}
 K(pn+1) 
 = \frac{L}{\sqrt{p}\eps}(pn+1)
 = \frac{L}{\eps}\left(\sqrt{p}n+\frac{1}{\sqrt{p}}\right)
 \geq \frac{2L\sqrt{n}}{\eps}
 \end{align*}
 where the equality holds when $p=1/n$. 
 \paragraph{Case 2:} If $\eps\geq L/\sqrt{n}$, L-SVRE with $K$ iterations holds that
 \begin{align*}
     {\rm Gap} \leq \frac{L}{\sqrt{p}K} \leq \frac{\sqrt{n}\eps}{\sqrt{p}K}
 \end{align*}
 We hope ${\rm Gap} \leq \eps$ which requires 
 \begin{align*}
  K\geq \sqrt{\frac{n}{p}}
 \end{align*}
 Then the total SFO complexity is at least
 \begin{align*}
 K(pn+1) 
 = \sqrt{\frac{n}{p}}(pn+1)
 = \left(\sqrt{p}n^{3/2}+\sqrt{\frac{n}{p}}\right)
 \geq 2n
 \end{align*}
 where the equality holds when $p=1/n$.

 \section{CSC}

 Our bound is 
 \begin{align}
     \fO\left(n + \sqrt{n L \kappa_y/\eps} + n^{3/4} \sqrt{\kappa_y} + n^{3/4}\sqrt{L/\eps}\right)
 \end{align}
 \citet{yang2020catalyst}'s bound is
 \begin{align*}
     \fO\left(\kappa_y L/\sqrt{\mu\eps} + n^{3/4}\sqrt{L/\eps}\right)
 \end{align*}
 If $\kappa>\sqrt{n}$, we have
 \begin{align*}
 \kappa_y L/\sqrt{\mu\eps} \geq \sqrt{n L \kappa_y/\eps}
 \end{align*}
 If $\kappa<\sqrt{n}$, we have
 \begin{align*}
 \kappa_y L/\sqrt{\mu\eps} \leq n^{3/4}\sqrt{L/\eps}
 \Longrightarrow  \fO\left(\kappa_y L/\sqrt{\mu\eps} + n^{3/4}\sqrt{L/\eps}\right) = \fO\left(n^{3/4}\sqrt{L/\eps}\right)
 \end{align*}
